# Supplementary material for: Cascaded Dual Vision Transformer for Accurate Facial Landmark Detection
Source: arXiv:2411.07167 source file (2025-12-17)
Supplement: Supplementary file 2 [file 10_appendix.tex]

\clearpage
\setcounter{page}{1}
\maketitlesupplementary

\section{GPU Memory Requirement}
 In ~\cref{table:memory} we report the memory required for each GPU during training, and number of parameters with different number of prediction blocks.

\begin{table}[htbp]
\centering
\begin{tabular}{l|llllll}
\toprule
\#Pred. Blocks & 2    & 4    & 6    & 8    & 10    & 12    \\
\midrule
Memory(GB)     & 4.4  & 6.3  & 8.2  & 10.3 & 12.1  & 14.2  \\
\#Param.(M)       & 24.4 & 48.4 & 72.4 & 96.4 & 120.4 & 144.4\\
\bottomrule
\end{tabular}
\caption{Memory required for each GPU during training, and number of parameters with different number of prediction blocks.}\label{table:memory}
\end{table}

\section{Compared to previous SOTA with similar computational capacity}
Our proposed Long Skip Connection enables the network to have more prediction blocks for accuracy. However, improved performance is not only attributed to in
creased computational capacity. When we use 4 prediction blocks and reduce the dimension of the feature maps
to (160, 32, 32), the parameter number of our network is
comparable to other baselines. As reported in ~\cref{tbl:param}, the
NME score still surpasses the previous SOTA by 0.08, and
this shows the effectiveness of our proposed architecture.

\begin{table}[htbp]

\centering
\small

\begin{tabular}{c|c|ccc}
\toprule
Method             & Params (M) & NME$(\downarrow)$  & Fr$_{10}(\downarrow)$   & AUC$_{10}(\uparrow)$   \\
\midrule
HIH                & 22.7       & 4.08 & 2.60 & 60.5  \\
SPIGA              & 60.3          & 4.06 & \textcolor{red}{2.08} & 60.6  \\
StarLoss           & 13.4       & 4.02 & \textcolor{blue}{2.32} & 60.5  \\
LDEQ               & 21.8       & \textcolor{blue}{3.92} & 2.48 & \textcolor{blue}{62.4}  \\
Ours\_nstack4 & 21.0       & \textcolor{red}{3.84} & 2.44 & \textcolor{red}{63.3} \\
\bottomrule
\end{tabular}
\caption{Comparisons on WFLW data set. We reduce the parameter number of network to 21M. Our proposed method still shows effectiveness.}\label{tbl:param}
\end{table}

\section{Evaluation on Different Image Resolution}
We test the influence of different input image resolutions. The results  with different prediction blocks are shown in ~\cref{fig:imagesize}. Specifically, D-VIT improves the performance by 0.09, 0.08 and 0.07 in 64px, 128px and 256px, respectively.  It means  our proposed method is not sensitive to input image size.
\begin{figure}[htbp]
  \centering
  \includegraphics[width=0.9\linewidth]{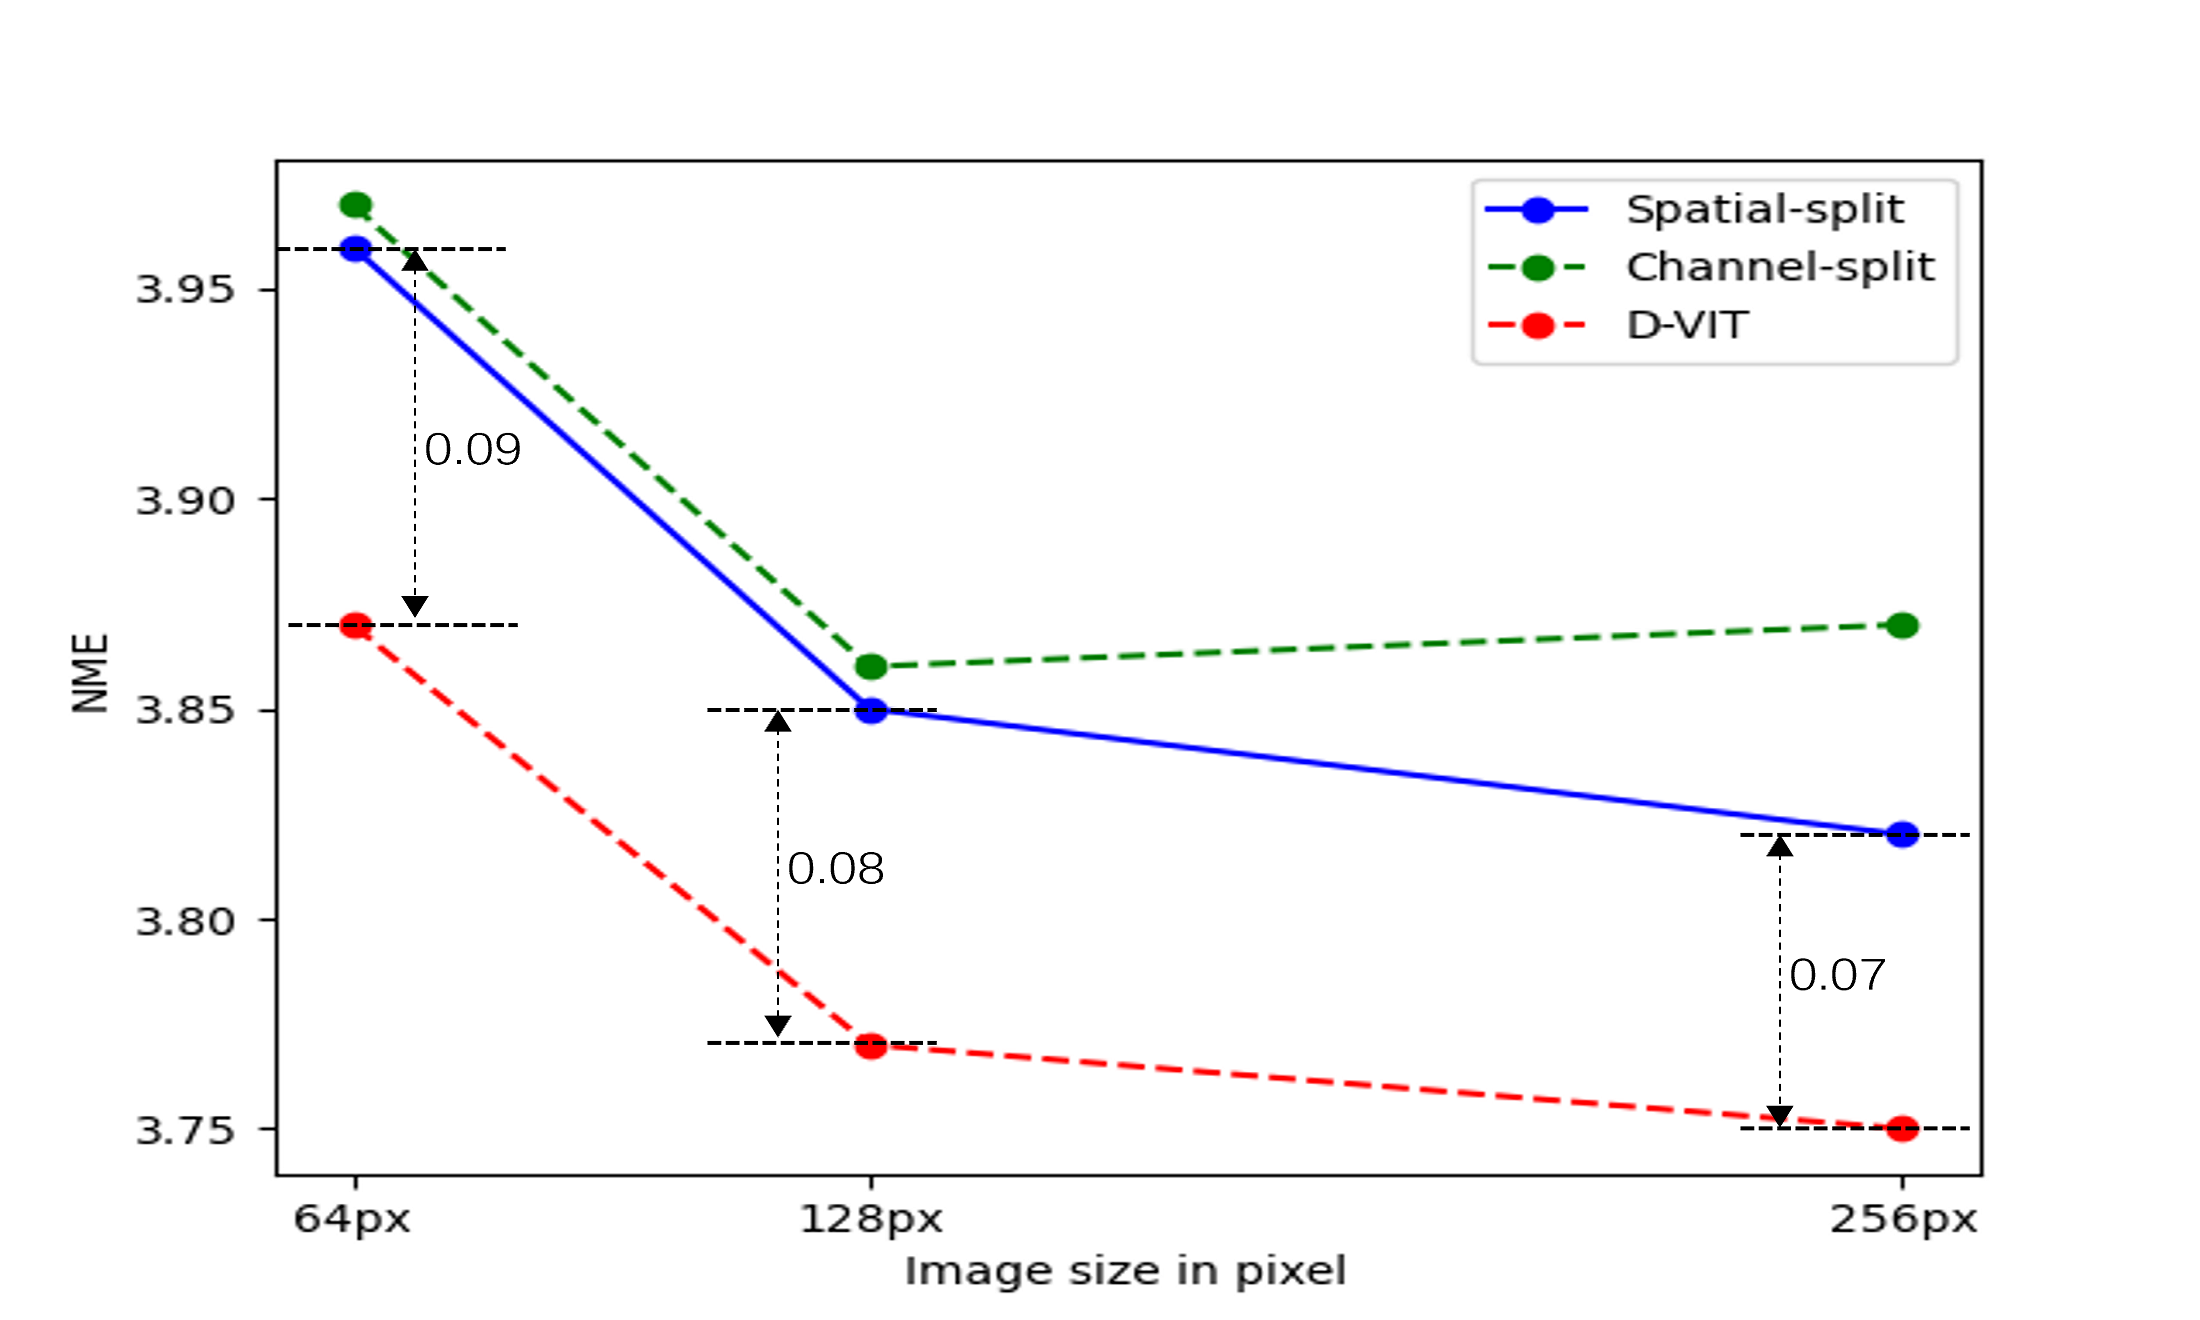}
\caption{NME against different input image size on WFLW dataset.}\label{fig:imagesize}
\end{figure}

\section{Quantitative results of different number of prediction blocks}
We report the numerical results on WFLW by using different number of prediction blocks in ~\cref{table:different_pred_blk}. The scores of NME, FR$_{10}$ and AUC$_{10}$ are reported on the whole test set and each sub set.

\begin{table*}[htbp]
\tiny
\negthinspace
\begin{tabular}{c|c|c|c|c|c|c|c}
\toprule
\#Block & FULL             & Pose              & Expr.            & Illum.           & Makeup           & Occlusion        & Blur             \\
\midrule
2           &\textls[-25]{3.88, 2.56, 63.0}&\textls[-25]{6.69, 11.04, 38.9}&\textls[-25]{3.92, 1.91, 61.9}&\textls[-25]{4.11, 1.72, 64.2}&\textls[-25]{3.73, 0.97, 64.5}&\textls[-25]{4.77, 4.89, 55.6}&\textls[-25]{4.57, 2.98, 57.7} \\
4            &\textls[-25]{3.81, 1.92, 63.2}&\textls[-25]{6.55, 9.20, 39.8 }&\textls[-25]{3.94, 1.59, 61.9}&\textls[-25]{3.98, 1.72, 64.4}&\textls[-25]{3.60, 2.43, 64.6}&\textls[-25]{4.66, 4.35, 55.9}&\textls[-25]{4.42, 2.33, 58.2} \\
6            &\textls[-25]{3.77, 1.72, 63.7}&\textls[-25]{6.59, 7.98, 39.9 }&\textls[-25]{3.82, 1.27, 62.9}&\textls[-25]{4.11, 1.29, 64.9}&\textls[-25]{3.64, 1.46, 64.7}&\textls[-25]{4.56, 3.40, 56.9}&\textls[-25]{4.40, 1.94, 58.8} \\
8            &\textls[-25]{3.75, 1.76, 63.7}&\textls[-25]{6.43, 8.28, 40.1 }&\textls[-25]{3.85, 1.27, 62.6}&\textls[-25]{4.06, 1.29, 64.7}&\textls[-25]{3.57, 1.94, 64.7}&\textls[-25]{4.47, 3.80, 57.1}&\textls[-25]{4.37, 2.07, 58.6}\\
\bottomrule
\end{tabular}
\caption{NME, FR$_{10}$, and AUC$_{10}$ score with different number of prediction blocks on WFLW dataset. The scores on sub sets are also included. As the number of prediction blocks increases, the NME score decreases. }\label{table:different_pred_blk}
\end{table*}

\section{Visual Results on COFW and 300W}
In this section we present the qualitative comparison results on COFW and 300W. ~\cref{fig:cofw:pred_blk} and  ~\cref{fig:300w:pred_blk} show the results of different prediction blocks. ~\cref{fig:cofw:conn} and ~\cref{fig:300w:conn} show the comparisons of different skip connection methods.  With the help of our proposed D-VIT  and LSC, the accuracy of predicted landmarks are improved.

\begin{figure}[htbp]
\centering
    \captionsetup[subfigure]{labelformat=empty}
    \begin{subfigure}{0.33\linewidth}
        \includegraphics[width=\linewidth]{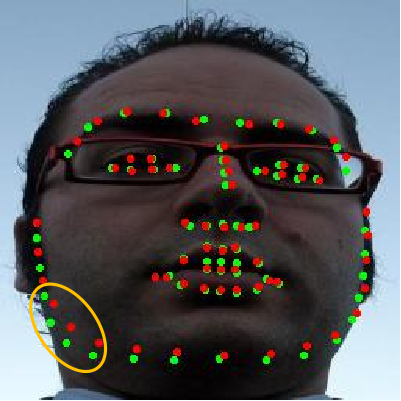}
    \end{subfigure}\hspace{-1mm}
    \begin{subfigure}{0.33\linewidth}
        \includegraphics[width=\linewidth]{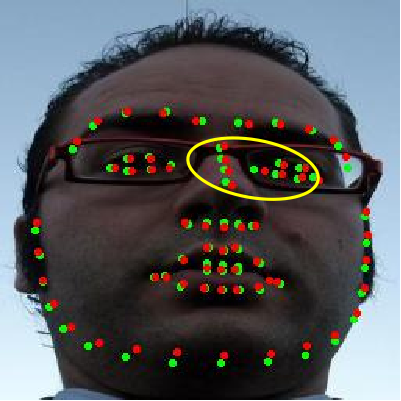}
    \end{subfigure}\hspace{-1mm}
    \begin{subfigure}{0.33\linewidth}
        \includegraphics[width=\linewidth]{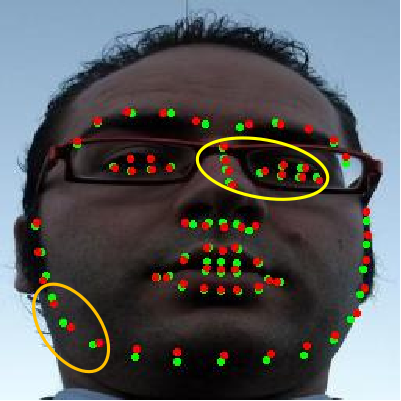}
    \end{subfigure}\vspace{-1mm}
    
    \begin{subfigure}{0.33\linewidth}
        \includegraphics[width=\linewidth]{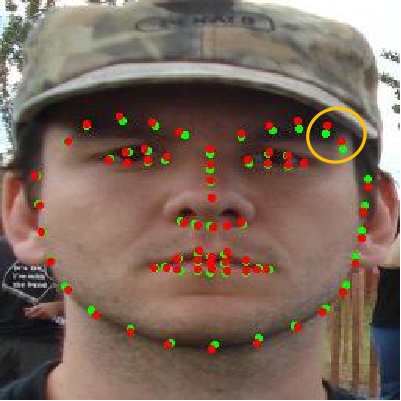}
        \caption{Spatial-split}
    \end{subfigure}\hspace{-1mm}
    \begin{subfigure}{0.33\linewidth}
        \includegraphics[width=\linewidth]{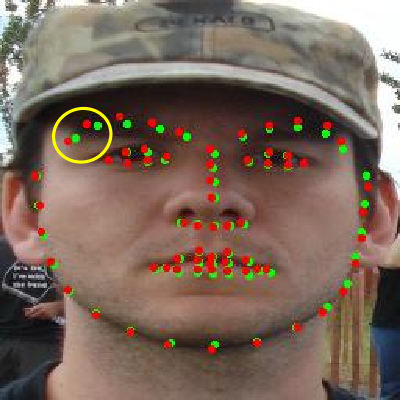}
        \caption{Channel-split}
    \end{subfigure}\hspace{-1mm}
    \begin{subfigure}{0.33\linewidth}
        \includegraphics[width=\linewidth]{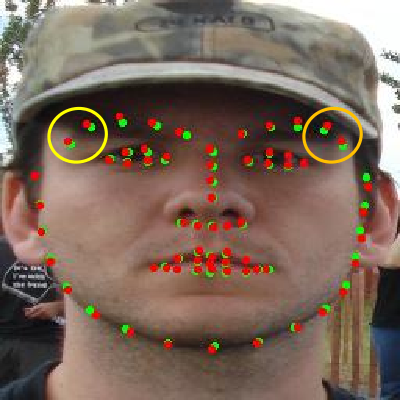}
        \caption{D-VIT}
    \end{subfigure}
    \caption{Visual comparison of different prediction blocks on 300W. Green and red points represent the predicted and ground-truth
landmarks, respectively.}\label{fig:300w:pred_blk}
\end{figure}

\begin{figure}[htbp]
\centering
    \captionsetup[subfigure]{labelformat=empty}
    \begin{subfigure}{0.33\linewidth}
        \includegraphics[width=\linewidth]{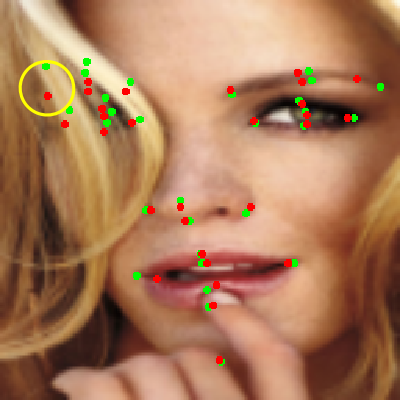}
    \end{subfigure}\hspace{-1mm}
    \begin{subfigure}{0.33\linewidth}
        \includegraphics[width=\linewidth]{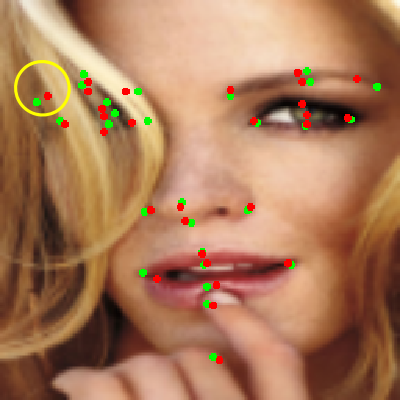}
    \end{subfigure}\hspace{-1mm}
    \begin{subfigure}{0.33\linewidth}
        \includegraphics[width=\linewidth]{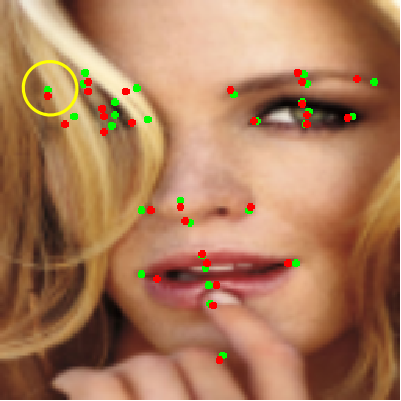}
    \end{subfigure}\vspace{-1mm}
    
    \begin{subfigure}{0.33\linewidth}
        \includegraphics[width=\linewidth]{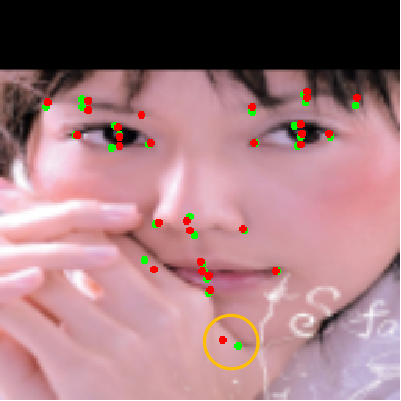}
        \caption{Spatial-split}
    \end{subfigure}\hspace{-1mm}
    \begin{subfigure}{0.33\linewidth}
        \includegraphics[width=\linewidth]{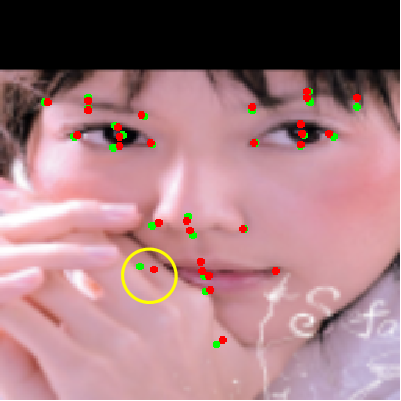}
        \caption{Channel-split}
    \end{subfigure}\hspace{-1mm}
    \begin{subfigure}{0.33\linewidth}
        \includegraphics[width=\linewidth]{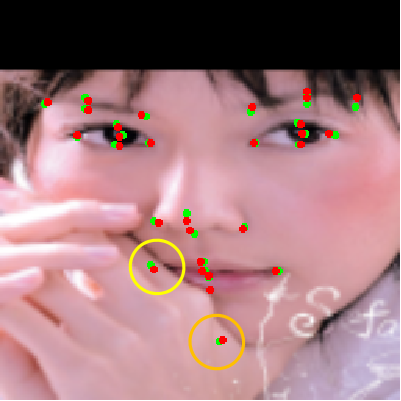}
        \caption{D-VIT}
    \end{subfigure}
    \caption{Visual results on the COFW dataset where contains heavy occlusions. To predict the landmark on occluded parts(orange and yellow circles) the spacial relations play an import role in boosting performance.  With the help of D-VIT our model learns the spatial relations among landmarks and is able to predict more accurately when occlusion happens.}\label{fig:cofw:pred_blk}
\end{figure}

\begin{figure}[htbp]
\centering
    \captionsetup[subfigure]{labelformat=empty}
    \begin{subfigure}{0.33\linewidth}
        \includegraphics[width=\linewidth]{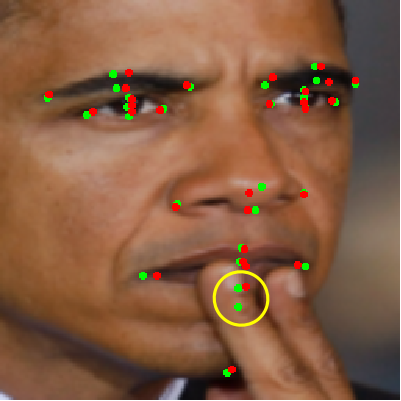}
    \end{subfigure}\hspace{-1mm}
    \begin{subfigure}{0.33\linewidth}
        \includegraphics[width=\linewidth]{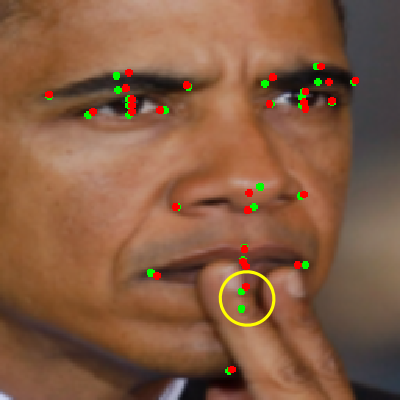}
    \end{subfigure}\hspace{-1mm}
    \begin{subfigure}{0.33\linewidth}
        \includegraphics[width=\linewidth]{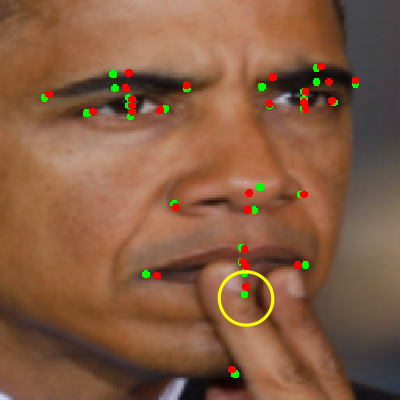}
    \end{subfigure}\vspace{-1mm}
    
    \begin{subfigure}{0.33\linewidth}
        \includegraphics[width=\linewidth]{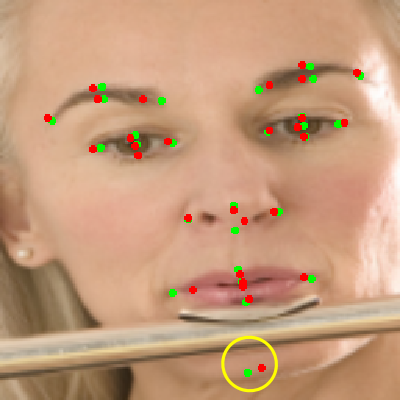}
        \caption{ResCBSP}
    \end{subfigure}\hspace{-1mm}
    \begin{subfigure}{0.33\linewidth}
        \includegraphics[width=\linewidth]{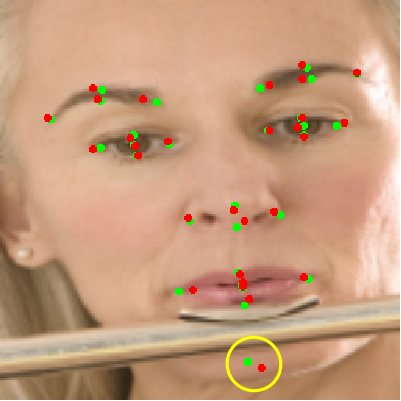}
        \caption{DenC}
    \end{subfigure}\hspace{-1mm}
    \begin{subfigure}{0.33\linewidth}
        \includegraphics[width=\linewidth]{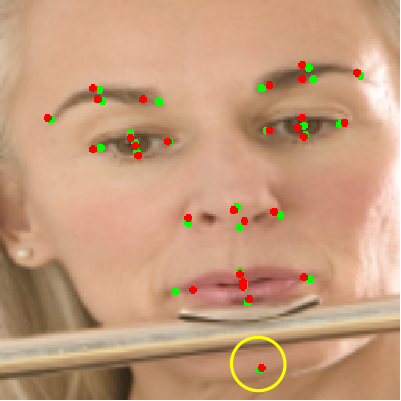}
        \caption{LSC}
    \end{subfigure}
    \caption{Qualitative results of different skip connection methods on COFW by using 8 prediction blocks. Green and red points represent the predicted and ground-truth
landmarks, respectively.}\label{fig:cofw:conn}
\end{figure}

\begin{figure}[htbp]
\centering
    \captionsetup[subfigure]{labelformat=empty}

    \begin{subfigure}{0.33\linewidth}
        \includegraphics[width=\linewidth]{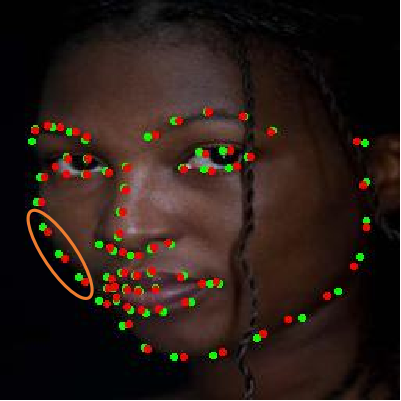}
    \end{subfigure}\hspace{-1mm}
    \begin{subfigure}{0.33\linewidth}
        \includegraphics[width=\linewidth]{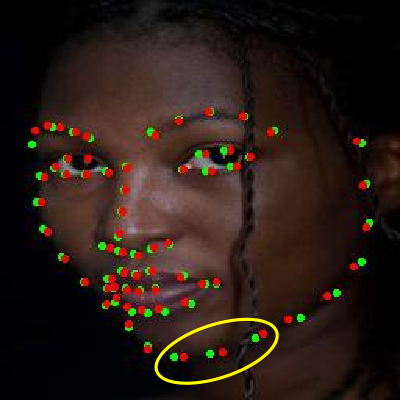}
    \end{subfigure}\hspace{-1mm}
    \begin{subfigure}{0.33\linewidth}
        \includegraphics[width=\linewidth]{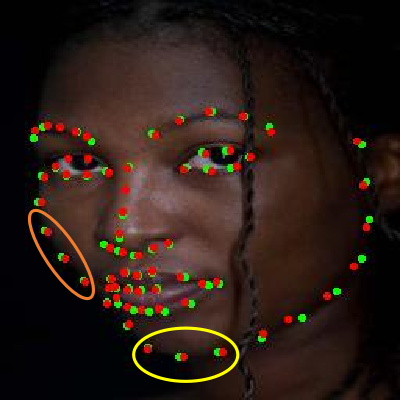}
    \end{subfigure}\vspace{-1mm}
    
    \begin{subfigure}{0.33\linewidth}
        \includegraphics[width=\linewidth]{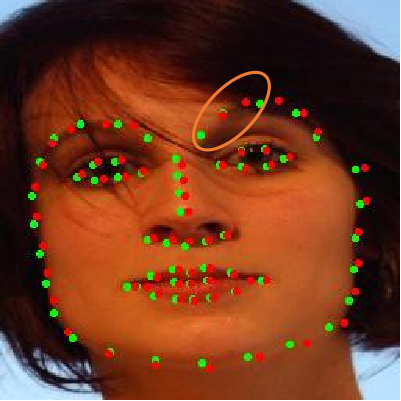}
        \caption{ResCBSP}
    \end{subfigure}\hspace{-1mm}
    \begin{subfigure}{0.33\linewidth}
        \includegraphics[width=\linewidth]{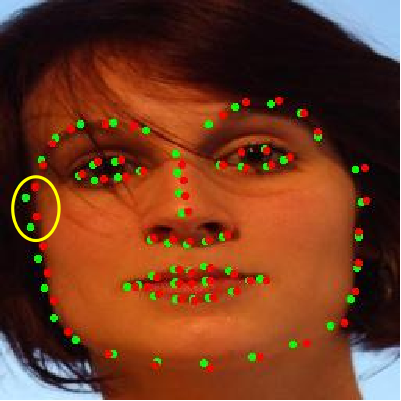}
        \caption{DenC}
    \end{subfigure}\hspace{-1mm}
    \begin{subfigure}{0.33\linewidth}
        \includegraphics[width=\linewidth]{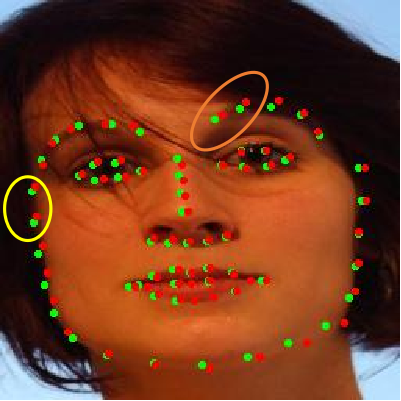}
        \caption{LSC}
    \end{subfigure}
    \caption{Qualitative results of different skip connection methods on 300W by using 8 prediction blocks. Green and red points represent the predicted and ground-truth
landmarks, respectively.}\label{fig:300w:conn}
\end{figure}
